# Supplementary material for: Dynamic Net Metering for Energy Communities
Source: arXiv:2306.13677 source file (2024-01-16)
Supplement: Supplementary file 1 [file AppendixCostCausationAxioms.tex]

We generalize the axiomatic community pricing to ensure fairness and efficiency \cite{Chakraborty&Poolla&Varaiya:19TSG,Shapley&Shubik:73RAND}.  In particular, we are interested in community pricing and payment rules that satisfy the axioms of 1) {\em individual rationality}, 2) {\em profit-neutrality}, 3) {\em \tcb{uniformity of payment}}, 4) {\em monotonicity}, and 5) {\em cost-causation penalty and cost-mitigation rewards}.

\begin{axiom}[Individual rationality]\label{ax:rationality}
    The surplus of every $i \in \mathcal{N}$ community member should be no less than its benchmark surplus -- i.e., $S^{\chi}_i(\bm{d}^\psi_i,z^\psi_i) \geq S_{i}^{\pi}\left(\bm{d}^\ast_i,z^\ast_i\right)=:S_{i}^{\ast,\pi}, \forall i \in \mathcal{N}$, where $(\bm{d}^\psi_i,z^\psi_i)$ and $(\bm{d}^\ast_i,z^\ast_i)$ are the optimal scheduling policies of community members and the benchmark, respectively.
\end{axiom}
\begin{axiom}[Profit-neutrality]\label{ax:ProfitNeutrality}
     The market mechanism must ensure the operator's profit-neutrality, i.e., $\Psi_\mathcal{N}^{\pi,\chi}=0$.
\end{axiom}
\begin{axiom}[\tcb{Uniformity of payment}]\label{ax:equity}
    The market mechanism has a \tcb{ uniform payment} if, for any two community members $i,j \in \mathcal{N}, i\neq j$, having $z_i =z_j$ results in $P^{\chi}_i(z_i)=P^{\chi}_j(z_j)$. \tcb{In the parlance of game theory, this is also called equal treatment of equals}.
\end{axiom}

\begin{axiom}[Monotonicity]\label{ax:monotonicity}
    The market mechanism is {\em monotonic} if, for any two community members $i,j \in \mathcal{N}, i\neq j$, having $|z_i| \geq |z_j|$ and $z_i z_j \geq 0$ result in $|P^{\chi}_i(z_i)|\geq |P^{\chi}_j(z_j)|$.
\end{axiom}
For axiom \ref{ax:CostCause}, the following definition is needed.
\begin{definition}[Cost causation and cost mitigation]\label{def:CostCausationMitigation}
    For every $i \in \mathcal{N}$, a net-consuming community member $z_i>0$ causes cost, whereas a net-producing community member $z_i <0$ mitigates cost.
\end{definition}
\begin{axiom}[Cost causation penalty and cost mitigation reward]\label{ax:CostCause}
A net-consuming member $z_i>0$ is penalized for causing cost and a net-producing member $z_i<0$ is rewarded for mitigating cost, i.e., for any $i\in \mathcal{N}, z_i\cdot P^{\chi}_i(z_i)\geq 0$.
\end{axiom}

\begin{definition}[Cost-causation principle]\label{def:CausationPrinciple}
    A community pricing rule $\chi^\sharp$ conforms with the {\em cost causation principle} if $\chi^\sharp \in \mathcal{C}:=\{\chi: \text{Axioms \ref{ax:rationality}--\ref{ax:CostCause} are satisfied}\}$.
\end{definition}

Note that the slight difference between the cost-causation principle defined above and that in \cite{Chakraborty&Poolla&Varaiya:19TSG} is the use of {\em surplus} rather than {\em payment} in {\em individual rationality}. Satisfying the cost-causation principle defined above implies satisfying that defined in \cite{Chakraborty&Poolla&Varaiya:19TSG}, but not vice versa.
